# Supplementary material for: Evolution of family systems and resultant socio-economic structures
Source: arXiv:2009.11035 source file (2021-10-01)
Supplement: Supplementary file 1 [file supplemantary.pdf]

# Supplementary Information for Evolution of family systems and resultant socio-economic structures

KENJI ITAO[1] AND KUNIHIKO KANEKO[1, 2, *]

[1] *Department of Basic Science, Graduate School of Arts and Sciences, University of Tokyo, Komaba 3-8-1, Meguro-Ku, Tokyo 153-8902, Japan.*
[2] *Research Center for Complex Systems Biology, University of Tokyo, Komaba 3-8-1, Meguro-Ku, Tokyo 153-8902, Japan.*
[*] *kaneko@complex.c.u-tokyo.ac.jp*

## SUPPLEMENTARY TEXT

### The Extended Model with Marriage Process

To consider the marriage process, each family has a population of sons and daughters (instead of asexual children in the minimal model). Concomitantly, the strategy parameter $\theta$ for the inheritance distribution between sons and daughters is introduced so that sons inherit $\theta/(1-\theta)$ times more than daughters, where $\theta$ values are set between 0 and 1. The values $\theta = 0, 0.5$, and 1 represent the states in which daughters inherit exclusively, sons and daughters inherit equally, and sons inherit exclusively, respectively. If there are $n$ sons and $m$ daughters in a family, the inheritance of $i$th son is proportional to

$$\frac{n\theta}{n\theta + m(1-\theta)} \cdot \frac{e^{-\lambda i}}{\sum_{k=1}^{n} e^{-\lambda k}}, \tag{S1}$$

whereas that of $j$th daughter is proportional to

$$\frac{m(1-\theta)}{n\theta + m(1-\theta)} \cdot \frac{e^{-\lambda j}}{\sum_{k=1}^{m} e^{-\lambda k}}. \tag{S2}$$

Marriage takes place before agricultural production. Male and female are randomly matched. If the sum of their wealth can afford the wealth required to support a wife $\epsilon_b$, they get married. Here, the wealth required for survival $\epsilon$ is paid at the timing of men's independence from parental family, whereas that required for marriage $\epsilon_b$ is paid at the timing of each marriage. If men can support additional wives, polygyny can occur. Polyandry can occur if brothers in the same extended family get one wife only.

In every family, daughters inherit some wealth and become independent before marriage. Sons in nuclear families inherit some wealth before marriage and each pays for marriage by himself, whereas for sons in extended families, the payment is funded from parental wealth. When sons in extended families get multiple wives, each son gets one wife in the order from the eldest. Then, if the number of wives exceeds that of sons, the eldest gets all additional wives.

The production is proportional to the logarithm of the number of husbands and wives in a family. Then, men in extended families inherit some wealth and leave the parental home with their wives. Families having at least one wife move into the reproduction process. When a family has $l$ wives, the numbers of sons and daughters follow the Poisson distribution with the mean $lb + fw$, where $b, f, w$ are the minimal birth rate, increment of birth rate by wealth, and family wealth, respectively. Thus, it is advantageous to have additional wives, since the number of children increases with the number of wives $l$. However, the number of children per wife is reduced to $b + fw/l$ as $l$ is increased. Such reduction of fitness is reported in empirical studies [1].

In the model of societies with labour-extensive subsistence patterns, the diminishing returns in labour input are relaxed. In this case, the production is proportional to the number of husbands and wives in a family. This corresponds to the situation where labour input is rather small compared to the capacity of resources such as land, and thus, diminishing returns are negligible.

### Deriving the Gamma Distribution from the Stochastic Process

In the wealth growth of our model, we consider the linear feedback from wealth and that from the logarithm of the labour force, as well as the multiplicative noise. Additionally, through the decay of wealth and the division of inheritance, the amount of wealth for each family is saturated. Here, wealth growth with positive feedback and nonlinear saturation with a multiplicative stochastic process is assumed.

The production of wealth increases with wealth $w$, which is generally saturated for large $w$. A simple example is given for the linear growth and the nonlinear saturation as $\dot{w} = aw - bw^2$, whereas the production rate fluctuates through the noise. Therefore, the simplest example of wealth dynamics is expressed as following Langevin equation (i.e. stochastic differential equation):

$$\dot{w} = aw - bw^2 + cw\eta, \tag{S3}$$

where the noise term $\eta$ follows a normal distribution. The stationary distribution P(w) of the Fokker-Planck equation (i.e. a partial differential equation for the time evolution of the probability density function) corresponding to Eq. (S3) is expressed as follows [2, 3]:

$$P(w) = \frac{1}{(cw)^2} \exp\left(2 \int \frac{aw - bw^2}{(cw)^2} dw\right) \tag{S4}$$

$$\propto \frac{1}{c^2 w^2} \exp\left(\frac{2a}{c^2} \log w - \frac{2b}{c^2} w\right) \tag{S5}$$

$$= \frac{w^{2(a/c^2-1)}}{c^2} \exp\left(-\frac{2b}{c^2} w\right). \tag{S6}$$

This defines the gamma distribution.

Our model includes a complicated process for the distribution of wealth among siblings and feedback from the labour force to wealth production, which cannot be written using simple forms, as shown in Eq. (S3). However, one may expect linear feedback, nonlinear saturation, and multiplicative stochasticity. Therefore, the simple model Eq. (S3) would capture the dynamics to a certain degree.

By comparing Eq. (S6) and the general form of the gamma distribution $w^\alpha \exp(-\beta w)$, the dependence of the wealth distribution on family systems is explained. The lightness of the poor tail $\alpha$ is smaller, i.e. there is a higher level of poverty, when the linear feedback rate from wealth to the production $a$ is smaller. Because labour efficiency per capita is smaller in extended families, $a$ is larger therein. (Strictly, $a$ is the largest for the eldest siblings in extended families, intermediate for siblings in nuclear families, and smallest for younger siblings in extended families. However, it is the wealth distribution of younger siblings that determines $\alpha$; hence, we can say $a$ is larger in nuclear families.) Thus, the poor tail is light in nuclear families, whereas it is heavy in extended families. The lightness of the rich tail $\beta$ is larger when the nonlinear saturation of wealth $b$ is larger. Equal inheritance prevents the accumulation of wealth, resulting in larger $b$. Hence, the rich tail is light in equal inheritance, whereas it is heavy in unequal inheritance. Hence, the trend shown in Figure 6 can be shown mathematically.

## SUPPLEMENTARY FIGURES

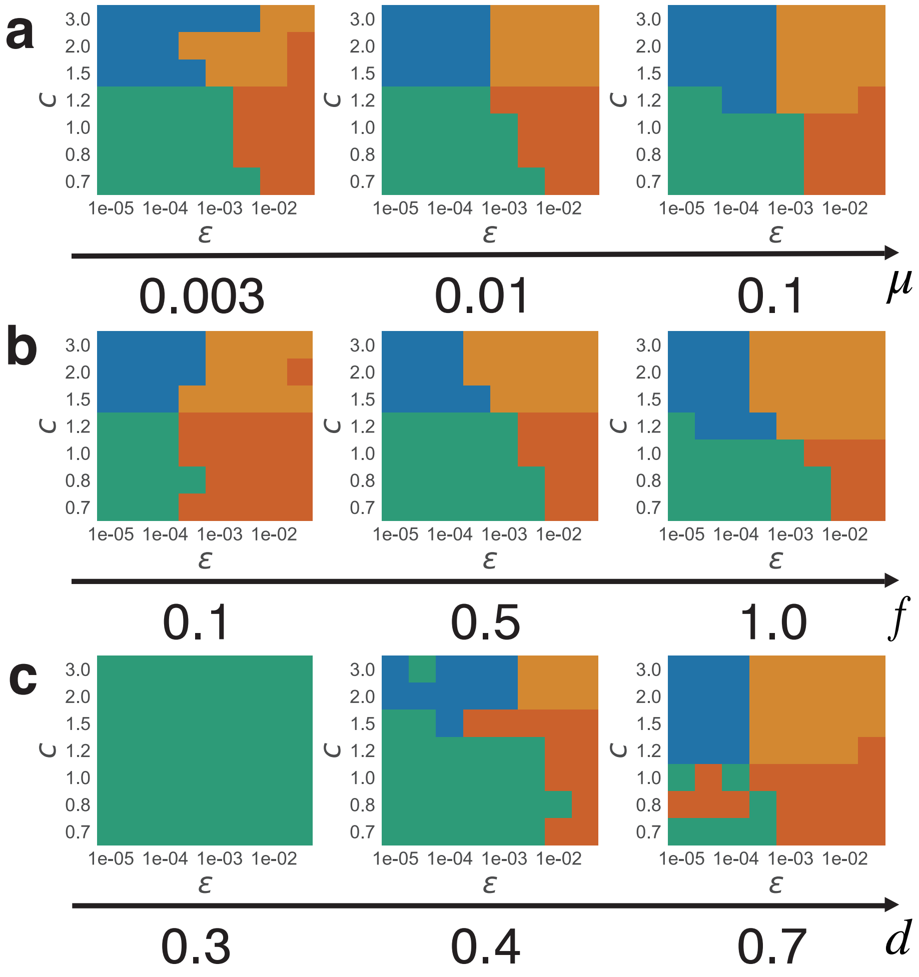


**Figure S1.** Dependence of phase diagrams of family systems on the parameters with $**$ in Table 1, i.e. mutation rate $\mu$, the increment of birth rate by wealth $f$, and decay rate of wealth $d$. Stem, community, absolute nuclear, and egalitarian nuclear families are plotted in green, orange, blue, and yellow, respectively. Unless the value is shown on the axis, the parameter values are fixed to those in Table 1. **a,** The dependence on mutation rate $\mu$. As $\mu$ gets larger, regions with nuclear families shown in blue and orange are enlarged. This is consistent with the general observation in multi-level evolution that a large mutation rate enables selfish strategies to evolve. **b,** The dependence on the increment of birth rate by wealth $f$. A large $f$ leads to a larger population for wealthy families. In extended families, a larger population provides greater production. Wealth accumulation is accelerated in extended families, and then, $\epsilon$ becomes relatively small for the wealth. It results in the development of unequal inheritance; thus, stem families replace community families. Additionally, a large $f$ results in many children. Therefore, family-level competition is intensified, and the regions of a nuclear family are enlarged. **c,** The dependence on the decay rate of wealth $d$. A large $d$ prevents wealth accumulation, and then, $\epsilon$ becomes relatively large for the wealth. It results in the development of equal inheritance. When $d$ is small, unequal inheritance develops. If it is too small, the nonlinear saturation of wealth accumulation works only weakly so that the wealth of stem families can reach $w \sim O(1000)$. At that time, the feedback from the wealth to the birth rate should be saturated, and our model assuming linear feedback would be invalid. There should be a biological upper limit to the number of offspring. For families with more wealth, higher-order negative feedback terms of wealth that are not considered here, will keep the fertility rate constant. Therefore, this model is only valid for $w \sim O(10)$. As long as $d \geq 0.4$, the nonlinear saturation works to keep $w \sim O(10)$, and the phase diagrams are qualitatively robust.

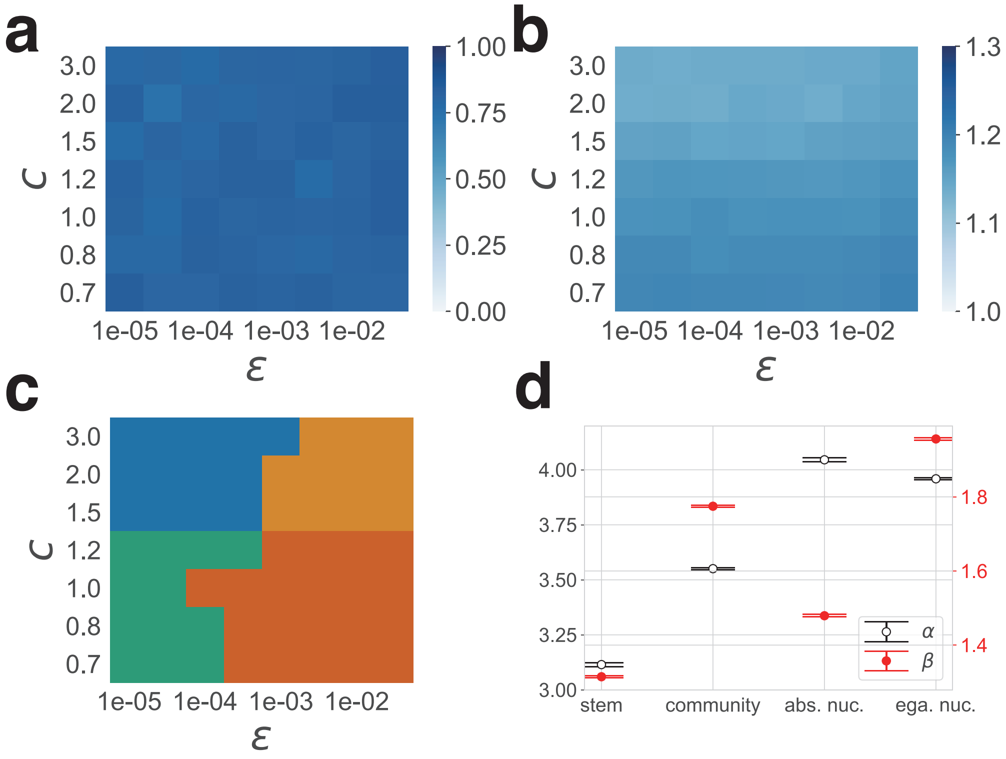


**Figure S2.** Simulation results of the extended model that includes the marriage process with discrimination between sons and daughters. Dependence of **a,** parental investment strategy $\theta$, and **b,** the average number of wives, **c,** family systems on environmental conditions, i.e. land capacity $c$ and wealth required for survival $\epsilon$, and that of **d,** the heaviness of the tails of the wealth distribution on family systems. **a,** The average value of parental investment strategy. The figure shows $\theta \simeq 0.8$, i.e. sons inherit almost 80 % of wealth on average, which means sons inherits four times as much as daughters. **b,** The average number of wives for married men. The frequency of polygyny is less than 20 % in most parameter regions. **c,** The phase diagram of family systems as in Figures 4c and S1. Stem, community, absolute nuclear, and egalitarian nuclear families are plotted in green, orange, blue, and yellow, respectively. The diagram is qualitatively robust against the implementation of the marriage process. **d,** Averaged value of the lightness of the poor tail $\alpha$ (black) and that of the rich tail $\beta$ (red) classified by the dominant family system (stem, community, absolute nuclear, and egalitarian nuclear families) in each society, with error bars. Values that are averaged over $\epsilon = 0.0001, 0.0003, 0.001, 0.003$ and $c = 1.0, 1.2, 1.5, 2.0$ are plotted. The dependence of the economic distribution on family systems is qualitatively the same as that of Figure 6. The wealth required to support a wife $\epsilon_b$ was set to 0.0001 in the simulation.

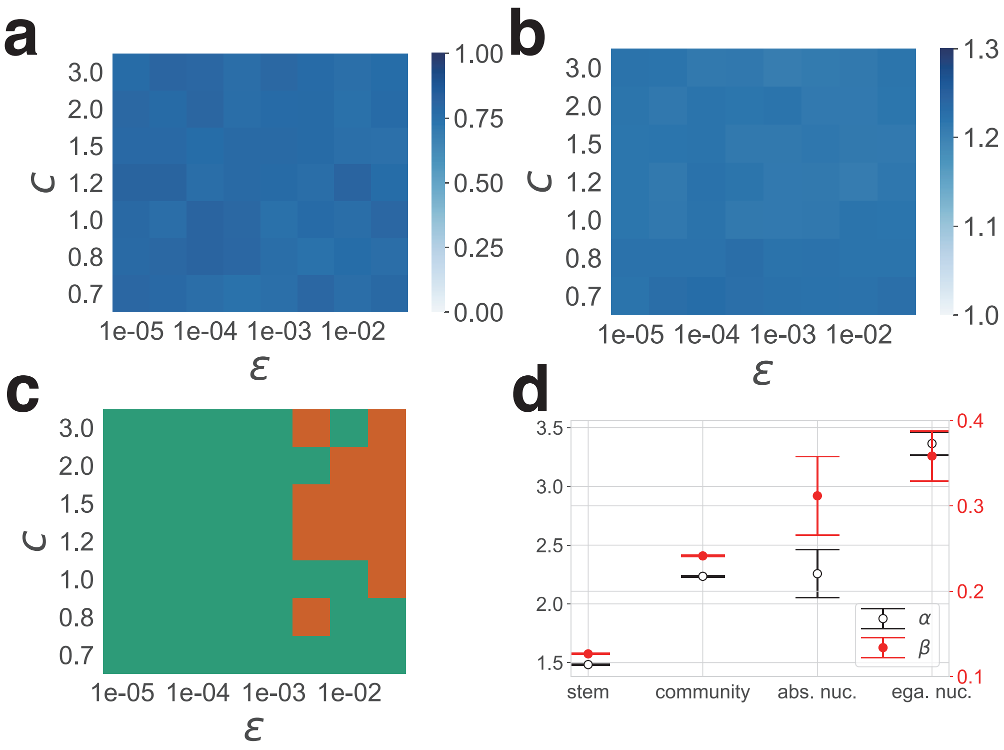


**Figure S3.** Simulation results of the extended model for the labour-extensive subsistence pattern in which the diminishing returns are relaxed and the production is proportional to labour input. Dependence of **a,** parental investment strategy $\theta$, **b,** the average number of wives, and **c,** family systems on environmental conditions, i.e. land capacity $c$ and wealth required for survival $\epsilon$, and that of **d,** the heaviness of the tails of the wealth distribution on family systems. **a,** The average value of parental investment strategy. The figure shows $\theta \simeq 0.8$, i.e. sons inherit almost 80 % of wealth on average, which means sons inherits four times as much as daughters. **b,** The average number of wives for married men. The frequency of polygyny is more than 20 % in most parameter regions which is larger than that for the model of agricultural societies. This is because, as shown in the following result **d**, the accumulation of wealth increases due to the lack of saturation in the labour force, which results in more families that are sufficiently rich to have multiple wives. **c,** The phase diagram of family systems as in Figures 4c and S1. Stem, community, absolute nuclear, and egalitarian nuclear families are plotted in green, orange, blue, and yellow, respectively. Extended families (plotted in green and orange) evolve in most parameter regions, because a nuclear family is no longer advantageous in productive efficiency. However, both nuclear and extended families are observed in other subsistence patterns. Even though extended families can be advantageous as productive units, nuclear families can evolve as households due to some reasons not covered by our model. **d,** Averaged value of the lightness of the poor tail $\alpha$ (black) and that of the rich tail $\beta$ (red) classified by the dominant family system (stem, community, absolute nuclear, and egalitarian nuclear families) in each society, with error bars. Values that are averaged over $\epsilon = 0.0001, 0.0003, 0.001, 0.003$ and $c = 1.0, 1.2, 1.5, 2.0$ are plotted. In this model, $\beta$ is much smaller for all family systems compared to those results for the model for agricultural society in Figures 6 and S3. Hence, the rich tails are heavier for all family systems here, which suggests that the fraction of relatively wealthy people is larger in such labour-extensive subsistence patterns. The wealth required to support a wife $\epsilon_b$ was set to 0.0001 in the simulation.

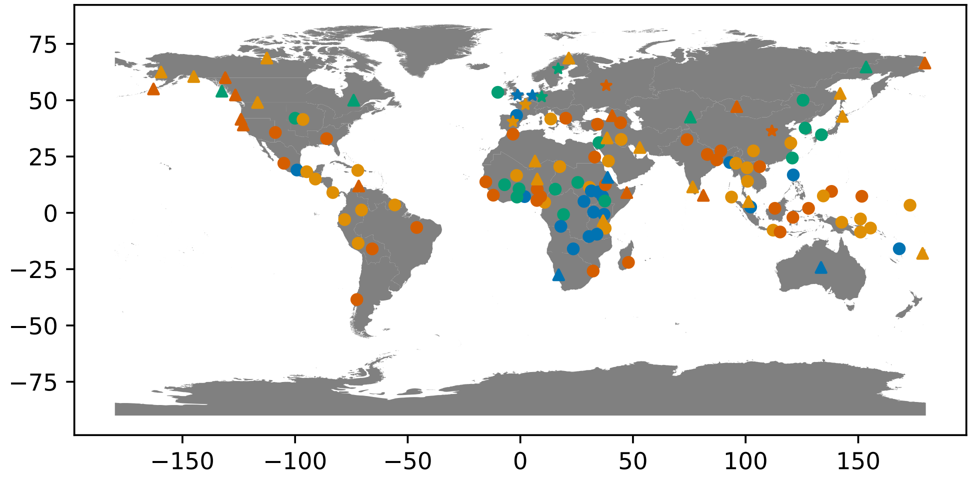


**Figure S4.** Geographic distribution of family systems. Stem, community, absolute nuclear, and egalitarian nuclear families are plotted in green, orange, blue, and yellow, respectively. Information about societies plotted with a circle (agricultural societies) and a triangle (other subsistence patterns) is based on the ethnographic database, Standard Cross-Cultural Sample (SCCS) [4, 5] and those plotted with a star is based on demographics by Todd [6]. In Eurasia, the regions close to the pole of civilisation such as China, India, and Mesopotamia conduct equal inheritance (orange and yellow), which may be explained by the frequent warfare therein. In contrast, unequal inheritance (green and blue) are observed in peripheral regions.

## SUPPLEMENTARY TABLES

**Table S1.** Correlation between variables in SCCS and parent–child relationship (whether nuclear or extended families). This table shows the variables that exhibit high correlation, together with their correlation and the average value of the variables for nuclear and extended families. The last column shows the p-value of correlation for each variable. The list shows the top 10 % of variables with high correlation (excerpt). Generally, a larger value of each item shows that a greater degree of the item is observed in the societies (e.g. larger value of SCCS956 shows that strong disapproval for infanticide in societies). Values of variables are explained in detail below. SCCS1082 shows that wage labour is more frequently introduced for nuclear families, as is consistent with economic histories in Western Europe [7]. SCCS762 shows that societies are more authoritarian if there are extended families. Furthermore, SCCS621 and SCCS626 show that male dominance is stronger for societies with extended families. These trends are consistent with the previous demographic study [8].

| Name | Explanation | Corr. | Nuclear | Extended | p |
|---|---|---|---|---|---|
| SCCS956 | Social (dis)approval for infanticide | 0.54 | 2.1 | 4.11 | 0.02 |
| SCCS1082 | Wage labour introduced | -0.40 | 0.5 | 0.14 | 0.01 |
| SCCS762 | (No) Removal of leaders who are incompetent or disliked | -0.38 | 2.69 | 2.06 | 0.04 |
| SCCS621 | (No) Explicit view that men dominate their wives | -0.38 | 1.67 | 1.19 | 0.03 |
| SCCS766 | (Low) Political participation | -0.36 | 3.19 | 2.55 | 0.02 |
| SCCS1776 | Frequency of intra-ethnic violence | -0.36 | 2.89 | 2.19 | 0.02 |
| SCCS626 | (No) Belief that women are generally inferior to men | -0.35 | 1.82 | 1.48 | 0.02 |
| SCCS910 | Collection of tribute | 0.35 | 1.69 | 1.95 | <0.01 |
| SCCS1262 | Occurrence of short-term starvation | 0.32 | 1.8 | 2.0 | <0.01 |
| SCCS1726 | Communality of land | -0.31 | 2.36 | 1.85 | 0.03 |
| SCCS1723 | Number of poor | 0.29 | 15.56 | 18.26 | 0.06 |
| SCCS876 | Polygyny distributions | 0.28 | 0.23 | 0.5 | 0.20 |
| SCCS1122 | Log10 of total population | 0.27 | 4.45 | 5.17 | 0.01 |
| SCCS1720 | Causes of land shortage | 0.26 | 1.29 | 1.55 | 0.09 |

**Table S2.** Correlation between variables in SCCS and inter-sibling relationship (whether strongly biased or equal inheritance). This table shows the variables that exhibit high correlation, together with their correlation and the average value of the variables for unequal and equal inheritance. The last column shows the p-value of correlation for each variable. The list shows the top 10 % of variables with high correlation (excerpt). SCCS1134, SCCS574, and SCCS1751 show that societies are more egalitarian if an equal inheritance is provided, which is consistent with the previous demographic study [8]. Here, we calculated the correlation between variables in SCCS with the inter-sibling relationship on the inheritance of movable property (SCCS281). However, the same analysis of the inter-sibling relationship on the inheritance of real property (SCCS280) shows a similar trend, especially for those variables related to the model parameters, for example, SCCS1721 (Corr. - 0.23) and SCCS1749 (Corr. 0.31).

| Name | Explanation | Corr. | Unequal | Equal | p |
|---|---|---|---|---|---|
| SCCS1134 | Despotic bias in conflict resolution | -0.58 | 1.56 | 1.04 | < 0.001 |
| SCCS570 | Fraternal interest group strength | -0.55 | 4.0 | 2.43 | < 0.001 |
| SCCS575 | Unstable political power index | 0.53 | 1.09 | 2.11 | <0.01 |
| SCCS1729 | Presence of an overarching political unit | 0.47 | 24.32 | 34.53 | <0.001 |
| SCCS1133 | Maximum harem size | -0.42 | 2.69 | 1.71 | 0.01 |
| SCCS954 | Social (dis)approval for abortion | -0.41 | 4.0 | 2.44 | 0.06 |
| SCCS574 | Achieved leadership through wealth distribution | 0.41 | 1.0 | 1.33 | 0.03 |
| SCCS953 | Contraception | 0.38 | 2.5 | 4.14 | 0.10 |
| SCCS1721 | Number of rich people (wealthy) | -0.37 | 18.68 | 15.67 | <0.01 |
| SCCS1749 | Frequency of internal warfare | 0.36 | 1.5 | 2.23 | 0.08 |
| SCCS918 | Manumission of slaves | 0.36 | 3.87 | 5.98 | <0.001 |
| SCCS794 | (Low) Female participation in private political arenas | -0.34 | 2.29 | 1.5 | 0.07 |
| SCCS1751 | Social stratification | -0.33 | 3.11 | 2.46 | 0.03 |
| SCCS1869 | Number of societies within 350 mile radius | -0.29 | 22.3 | 12.29 | <0.01 |
| SCCS782 | (Un) Acceptability of violence within society | -0.27 | 2.88 | 2.29 | 0.13 |

### Values of SCCS Variables Used for Data Analyses

The values of SCCS variables are explained as below, according to [4, 5, 9–24]

**SCCS246** ***Subsistence economy: dominant activity***
1. Gathering, 2. Fishing, 3. Hunting, 4. Pastoralism, 5. Casual agriculture, 6. Extensive agriculture, 7. Intensive agriculture, and 8. Two or more sources.

**SCCS210** ***Domestic organization***
1. Nuclear, monogamous, 2. Nuclear, limited polygyny, 3. Nuclear, polyandrous, 4. Nuclear, polygyny, atypical cowives pattern, 5. Nuclear, polygyny, typical cowives pattern, 6. Minimal extended, 7. Small extended, and 8. Large extended.

**SCCS280** ***Inheritance distribution for real property (land)***
1. Equally distributed, 2. Best qualified, 3. Ultimogeniture, 4. Primogeniture, and 9. No inheritance of real property.

**SCCS281** ***Inheritance distribution for movable property***
1. Equally distributed, 2. Best qualified, 3. Ultimogeniture, 4. Primogeniture, and 9. No inheritance of movable property.

**SCCS956** ***Social (Dis)approval for Infanticide***
1. Occurs but no data, 2. Permit & Frequent, 3. Permit & Infrequent, 4. Disapprove & Occurs, and 5. Disapprove & no Occur.

**SCCS1082** ***Wage Labour Introduced***
0. No, and 1. Yes.

**SCCS762** ***(No) Removal of Leaders Who Are Incompetent or Disliked***
1. No way other than rebellion or popular uprisings, 2. Institutionalized means invoked occasionally by elites, 3. Not removed in a formal manner, lose influence & are ignored, and 4. No formal leadership, loss of power when support diminishes.

**SCCS621** ***(No) Explicit View That Men Should and Do Dominate Their Wives***
1. Yes, 2. No, evidence of rough equality, and 3. No, evidence of wife dominance

**SCCS766** ***(Low) Political Participation: Extensivity of Adult Participation in Areas Where Collective Decision Making Present***
1. Widespread: decision-making forums open to all adults, 2. High or some: excluded basis on gender, age, or kinship, 3. Moderate: some consultation present, low input from community, and 4. Low or non-existent: Leaders make most decisions.

**SCCS1776** ***Frequency of Intraethnic Violence***
1. Rare or never, 2. Occasional, 3. Often, and 4. Permanent.

**SCCS626** ***(No) Belief That Women Are Generally Inferior to Men***
1. Yes, 2. No such belief.

**SCCS910** ***Collection of Tribute***
1. Present, and 2. Absent or not mentioned.

**SCCS1262** ***Occurrence of short-term starvation***
1. Low, 2. Moderate, and 3. High.

**SCCS1726** ***Communality of Land***
1. Land predominantly private property, 2. Land partially communally used, and 3. Communal land use rights only.

**SCCS1723** ***Number of Poor***
10. Absence of poor, 15. Few poor, 20. Presence of poor, and 25. Many poor. [1]

**SCCS876** ***Polygyny Distributions***
0. True Binomial, and 1. Negative Binomial.

[1] The original values were 10. Absence of poor, 20. Presence of poor, 21. Few poor, and 22. Many poor. Here, we arranged the values to make them positively correlated to the number of poor.

**SCCS1122** ***Log10 of Total Population***

1. 10-99, 2. 100-999, 3. 1,000-9,999, 4. 10,000-99,999, 5. 100,000-999,999, 6. 1,000,000-9,999,999, 7. 10,000,000-99,999,999, and 8. 100,000,000-999,999,999.

**SCCS1720** ***Causes of land shortage***

1. No land shortage, 2. Population pressure (caused by humans or animals), 3. Territorial invasions, and 4. More than one of the above.

**SCCS1134** ***Despotic Bias in Conflict Resolution***

1. Despotism absent: bias in the resolution of individual, 2. Despotism present: Conflicts of interest among individuals.

**SCCS570** ***Fraternal Interest Group Strength***

1. Both brideprice and patrilineality are absent, 2. Either brideprice or patrilineality, 3. Political subunit is greater than 1,000, brideprice present, 4. Size of the political subunit is between 100-999, 5. Political subunits greater than 1,000, brideprice absent.

**SCCS575** ***Unstable Political Power Index***

1. All three variables–ritual warfare, achieved leadership, and social indebtedness–have a score of 0, 2. Only one of the three variables has a score of 1, 3. Two of the variables have a score of 1, and 4. All three variables have a score of 1.

**SCCS1729** ***Presence of an Overarching Political Unit***

10. Local community autonomous, 20. Local community is part of a pre-colonial state, 21. Ethnic group to which the local community belongs is politically dominant in the pre-colonial state, 22. Ethnic group to which the local community belongs occupies a politically subordinate position in the pre-colonial state, 30. Local community is part of a colonial state, 40. Local community is part of a postcolonial state, 41. Ethnic group to which the local community belongs is politically dominant in the postcolonial state, and 42. Ethnic group to which the local community belongs occupies a politically subordinate position in the postcolonial state.

**SCCS1133** ***Maximum Harem Size***

1. 3 conjugal relationships or less, 2. 4-10 conjugal relationships, 3. 11-100 conjugal relationships, and 4. More than 100 conjugal relationships.

**SCCS954** ***Social Approval for Abortion: Approval of and Rationale for Action Taken to Prevent the Birth of a Child by Expelling the Fetus before It Is Viable***

1. Abortions occur, but there is no information on frequency, 2. Abortions are permitted and occur frequently, 4. Abortions are disapproved of but do occur, and 5. Abortions are strongly disapproved of and occur rarely or never.

**SCCS574** ***Achieved Leadership through Wealth Distribution***

1. Not important, and 2. Very important.

**SCCS953** ***Contraception: Knowledge and Use of Means to Prevent the Conception of Children***

1. No contraception is known about or used, 2. Contraception is present, but there is no information on the method, 3. There is a rudimentary form of contraception, 4. Contraception is present by implication, 5. There are long post-partum sex taboos and rudimentary contraception, 6. There are long post-partum sex taboos and the woman practices some intentional form of contraception, and 7. The woman is primarily responsible for contraception.

**SCCS1721** ***Number of Rich People (Wealthy)***

10. Absence of rich, 15. Few rich, 20. Presence of rich, 25. Many rich [2]

**SCCS1748** ***Frequency of Internal Warfare Involving Non-territorially Organized Groups within Unit of Maximal Political Authority***

1. Rare or never, 2. Occasional, 3. Often, 4. Permanent

[2]The original values were 10. Absence of rich, 20. Presence of rich, 21. Few rich, and 22. Many rich. Here, we arranged the values to make them positively correlated to the number of rich.

**SCCS918** ***Manumission of Slaves***

1. Infrequent, 2. Not common, 3. Frequent, 4. No data on rates of manumission, but hereditary slaveholding is present by Patterson's definition, 5. Hereditary slaveholding is not present by Patterson's definition, although present by Murdock's definition, 6. Hereditary slaveholding is not present by Patterson's definition, although slavery is present by Murdock's definition, unascertained as to whether hereditary, 7. Hereditary slaveholding is not present by Patterson's definition, although nonhereditary, slavery is present (e.g., slaves captured in warfare but not inherited) by Murdock's definition, 8. Slavery is not present by either definition, and 9. Slavery is not present by either definition, although the societies are largely composed of former slaves.

**SCCS794** ***(Low) Female Participation in Private Political Arenas, Relative to Males***

1. High: in some situations equal to or greater than that of men, 2. Significant but not as high as male involvement, 3. Not great but clearly some role for women in private aspects of political life, and 4. Women do not seem to get involved in political life in private arenas.

**SCCS1751** ***Social Stratification***

1. No differences in access to economic resources, political power, and/or status, 2. Differences in access to economic resources, political power, and/or status, not resulting in class formation, 3. Two classes, 4. Complex stratification into more than two classes

**SCCS1869** ***Concordance: Number of Societies within 350 Mile Radius***

Number of Societies within 350 Mile Radius

**SCCS782** ***(Un) Acceptability of Violence toward Members of the Same Society, but outside the Local Community***

1. Valued, 2. Acceptable, 3. Tolerated, and 4. Disapproved.

## REFERENCES


1. C. T. Ross, M. Borgerhoff Mulder, S.-Y. Oh, S. Bowles, B. Beheim, J. Bunce, M. Caudell, G. Clark, H. Colleran, C. Cortez *et al.*, "Greater wealth inequality, less polygyny: rethinking the polygyny threshold model," J. The Royal Soc. Interface **15**, 20180035 (2018).
2. H. Risken, *Fokker-planck equation* (Springer, 1996).
3. M. Suzuki, K. Kaneko, and F. Sasagawa, "Phase transition and slowing down in non-equilibrium stochastic processes," Prog. Theor. Phys. **65**, 828–849 (1981).
4. G. P. Murdock and D. R. White, "Standard cross-cultural sample," Ethnology **8**, 329–369 (1969).
5. K. R. Kirby, R. D. Gray, S. J. Greenhill, F. M. Jordan, S. Gomes-Ng, H.-J. Bibiko, D. E. Blasi, C. A. Botero, C. Bowern, C. R. Ember *et al.*, "D-place: A global database of cultural, linguistic and environmental diversity," PloS one **11**, e0158391 (2016).
6. E. Todd, *La diversité du monde: structures familales et modernité* (Seuil, 1999).
7. I. Wallerstein, *The modern world-system I: Capitalist agriculture and the origins of the European world-economy in the sixteenth century*, vol. 1 (Univ. of California Press, 2011).
8. E. Todd, *L'origine des systèmes familiaux*, vol. 1 (Gallimard Paris, 2011).
9. A. Seda, "Cross-cultural codes of modernization," World Cult. **11**, 152–170 (2000).
10. J. P. Gray, "A corrected ethnographic atlas," World Cult. **10**, 24–85 (1999).
11. G. P. Murdock, "Ethnographic atlas, installments i-xxvii," Ethnology pp. 1–10 (1962).
12. R. Dirks, "Starvation and famine: cross-cultural codes and some hypothesis tests," Cross-Cultural Res. **27**, 28–69 (1993).
13. B. S. Low, "Pathogen intensity cross-culturally," World Cult. **8**, 24–34 (1994).
14. K. E. Paige and J. M. Paige, *The politics of reproductive ritual* (Univ of California Press, 1981).
15. M. H. Ross, "Political decision making and conflict: Additional cross-cultural codes and scales," Ethnology **22**, 169–192 (1983).
16. W. Divale, N. Abrams, J. Barzola, E. Harris, and F. Henry, "Sleeping arrangements of children and adolescents: Sccs sample codes," World Cult. **9**, 3–12 (1998).
17. M. K. Whyte, "Cross-cultural codes dealing with the relative status of women," Ethnology **17**, 211–237 (1978).
18. H. Lang, "Conan: An electronic code-text data-base for cross-cultural studies," World Cult. **9**, 13–56 (1998).
19. C. Bradley, C. C. Moore, M. L. Burton, and D. R. White, "A cross-cultural historical analysis of subsistence change," Am. Anthropol. **92**, 447–457 (1990).
20. S. G. Frayser, *Varieties of sexual experience: An anthropological perspective on human sexuality* (HRAF Press, 1985).
21. E. Cashdan, "Ethnic diversity and its environmental determinants: Effects of climate, pathogens, and habitat diversity," Am. Anthropol. **103**, 968–991 (2001).
22. G. P. Murdock and S. F. Wilson, "Settlement patterns and community organization: Cross-cultural codes 3," Ethnology **11**, 254–295 (1972).
23. R. P. Rohner and E. C. Rohner, "Enculturative continuity and the importance of caretakers: Cross-cultural codes," Behav. Sci. Res. **17**, 91–114 (1982).
24. C. Bradley, "The household division of work: Sccs codes," World Cult. **8**, 6–36 (1994).
